# Supplementary material for: Native state of natural proteins optimises local entropy
Source: arXiv:2111.12987 ancillary file (2021-11-25)
Supplement: Supplementary file 1 [file suppMat.pdf]

# The native state of natural proteins optimises local entropy – Supplementary Material


M. Negri

*Department Applied Science and Technology, Politecnico di Torino, CorsoDuca degli Abruzzi 24, I-10129 Torino, Italy**

G. Tiana

*Department of Physics and Center for Complexity and Biosystems, Università degli Studi di Milano and INFN, via Celoria 16, 20133 Milano, Italy*†

R. Zecchina

*Artificial Intelligence Lab, Bocconi University, Via Sarfatti, 25, 20136 Milano, Italy*‡



(Dated: November 25, 2021)


| $\gamma$ | std($f_{\text{eq}}$) | std($\tau$) | median(MSE) | std(MSE) |
|---|---|---|---|---|
| $5.0 \cdot 10^2$ | $8.2239 \cdot 10^{-}2$ | $1.0669 \cdot 10^3$ | $2.7821 \cdot 10^{-}4$ | $1.5583 \cdot 10^{-}4$ |
| $2.0 \cdot 10^3$ | $1.3406 \cdot 10^{-}1$ | $8.9720 \cdot 10^2$ | $2.2772 \cdot 10^{-}4$ | $1.7510 \cdot 10^{-}4$ |
| $8.0 \cdot 10^3$ | $1.1693 \cdot 10^{-}1$ | $4.3120 \cdot 10^3$ | $1.8888 \cdot 10^{-}4$ | $1.0092 \cdot 10^{-}4$ |
| $2.5 \cdot 10^3$ | $7.5114 \cdot 10^{-}2$ | $2.2077 \cdot 10^3$ | $2.3513 \cdot 10^{-}4$ | $1.1705 \cdot 10^{-}4$ |
| $5.0 \cdot 10^3$ | $1.0108 \cdot 10^{-}1$ | $1.2295 \cdot 10^3$ | $2.8181 \cdot 10^{-}4$ | $2.1203 \cdot 10^{-}4$ |
| $6.0 \cdot 10^3$ | $1.0941 \cdot 10^{-}1$ | $2.6071 \cdot 10^3$ | $2.0890 \cdot 10^{-}4$ | $1.2907 \cdot 10^{-}4$ |
| $7.0 \cdot 10^3$ | $1.5255 \cdot 10^{-}1$ | $1.8627 \cdot 10^4$ | $3.0163 \cdot 10^{-}4$ | $2.1992 \cdot 10^{-}4$ |
| $9.0 \cdot 10^3$ | $1.2876 \cdot 10^{-}1$ | $2.1858 \cdot 10^3$ | $2.0844 \cdot 10^{-}4$ | $2.2282 \cdot 10^{-}4$ |
| $1.0 \cdot 10^4$ | $9.0906 \cdot 10^{-}2$ | $3.8539 \cdot 10^2$ | $2.4447 \cdot 10^{-}4$ | $1.1748 \cdot 10^{-}4$ |
| $1.1 \cdot 10^4$ | $8.6400 \cdot 10^{-}2$ | $4.3558 \cdot 10^2$ | $2.0593 \cdot 10^{-}4$ | $1.5520 \cdot 10^{-}4$ |
| $1.2 \cdot 10^4$ | $1.0607 \cdot 10^{-}1$ | $3.9646 \cdot 10^2$ | $2.6716 \cdot 10^{-}4$ | $1.1724 \cdot 10^{-}4$ |
| $1.3 \cdot 10^4$ | $1.3475 \cdot 10^{-}1$ | $6.4258 \cdot 10^2$ | $2.3607 \cdot 10^{-}4$ | $1.8014 \cdot 10^{-}4$ |
| $1.4 \cdot 10^4$ | $7.7247 \cdot 10^{-}2$ | $3.8472 \cdot 10^2$ | $3.0565 \cdot 10^{-}4$ | $1.3042 \cdot 10^{-}4$ |
| $1.5 \cdot 10^4$ | $9.7204 \cdot 10^{-}2$ | $2.9444 \cdot 10^2$ | $2.4793 \cdot 10^{-}4$ | $2.0832 \cdot 10^{-}4$ |
| $2.0 \cdot 10^4$ | $6.7892 \cdot 10^{-}2$ | $7.8561 \cdot 10^2$ | $2.8288 \cdot 10^{-}4$ | $1.4823 \cdot 10^{-}4$ |
| $3.0 \cdot 10^4$ | $8.9116 \cdot 10^{-}2$ | $6.2010 \cdot 10^2$ | $2.8535 \cdot 10^{-}4$ | $1.7384 \cdot 10^{-}4$ |

TABLE S1: **Folding times and stabilities are less variable for higher values of $\gamma$.** The first two columns of the table show standard deviation of stabilities and folding times shown in Fig. 2a of the main text. The last two columns show median and standard deviation of mean square error of fits averaged over the samples, attesting the goodness of the fits.

| $\gamma$ | cooperativity $\kappa$ |
|---|---|
| 0.0 | $1.21 \pm 0.01$ |
| $0.5 \cdot 10^4$ | $1.35 \pm 0.04$ |
| $1.0 \cdot 10^4$ | $1.28 \pm 0.03$ |
| $2.0 \cdot 10^4$ | $1.42 \pm 0.07$ |

TABLE S2: **Local entropy leads to less cooperative transitions.** The table shows the estimated average cooperativity of the coil globule transition for go models on references at various values of $\gamma$. The cooperativity is defined with the Privalov coefficient $\kappa$, that is 1 in case of perfect first-order transition and greater than one the less cooperative the transition is. The definition is $\kappa := \int dT C_v(T)/2T_f\sqrt{C_v(T)}$, where $T_f$ is the folding temperature and $C_v$ is the specific heath of the transition.


* matteo.negri@polito.it

† guido.tiana@unimi.it

‡ riccardo.zecchina@unibocconi.it

| Protein | Mean($E_{\rm tr}$) | Var($E_{\rm tr}$) | Mean($T_{\rm tr}$) | Var($T_{\rm tr}$) |
|---|---|---|---|---|
| 1pgb | 6.69 | 1.95 | 89.16 | 18.76 |
| 2abd | 7.73 | 1.60 | 88.76 | 14.75 |
| 2ci2 | 5.67 | 1.18 | 88.43 | 14.80 |
| HHH | 5.84 | 1.83 | 77.45 | 14.84 |
| 1bnr | 8.72 | 0.92 | 92.74 | 12.06 |
| 1cye | 9.81 | 4.40 | 107.24 | 32.00 |
| 5vnt | 7.40 | 1.65 | 83.81 | 12.13 |
| 1srl | 6.72 | 1.82 | 72.88 | 9.95 |

TABLE S3: **Average transition temperatures and corresponding transition energies.** We identified transition temperatures for each native and random structure as the position of the first peak in the specific heat (coming from high temperatures). The corresponding transition energy is determined with the energy curves shown in Fig. S8. We average those energies for each protein to determine the region where the transition states are in Fig. 3c-f in the main text. This "transition region" is plotted as a grey band.

| $\gamma$ | Tr $M^4$ | Tr $M^8$ | cont. range |
|---|---|---|---|
| 0.0 | $784.4 \pm 0.8$ | $41150 \pm 90$ | $19.28 \pm 0.05$ |
| $0.5 \cdot 10^4$ | $790.3 \pm 0.9$ | $41524 \pm 99$ | $19.80 \pm 0.05$ |
| $1.0 \cdot 10^4$ | $821.3 \pm 0.9$ | $44814 \pm 112$ | $17.96 \pm 0.05$ |
| $1.5 \cdot 10^4$ | $794.7 \pm 0.9$ | $42511 \pm 98$ | $16.81 \pm 0.04$ |

TABLE S4: **Properties of the contact map $M$ of lattice structures.** The table shows the fourth and eighth power of the contact map and the mean contact range as a function of $\gamma$. The quantities are averaged over 60 structures.

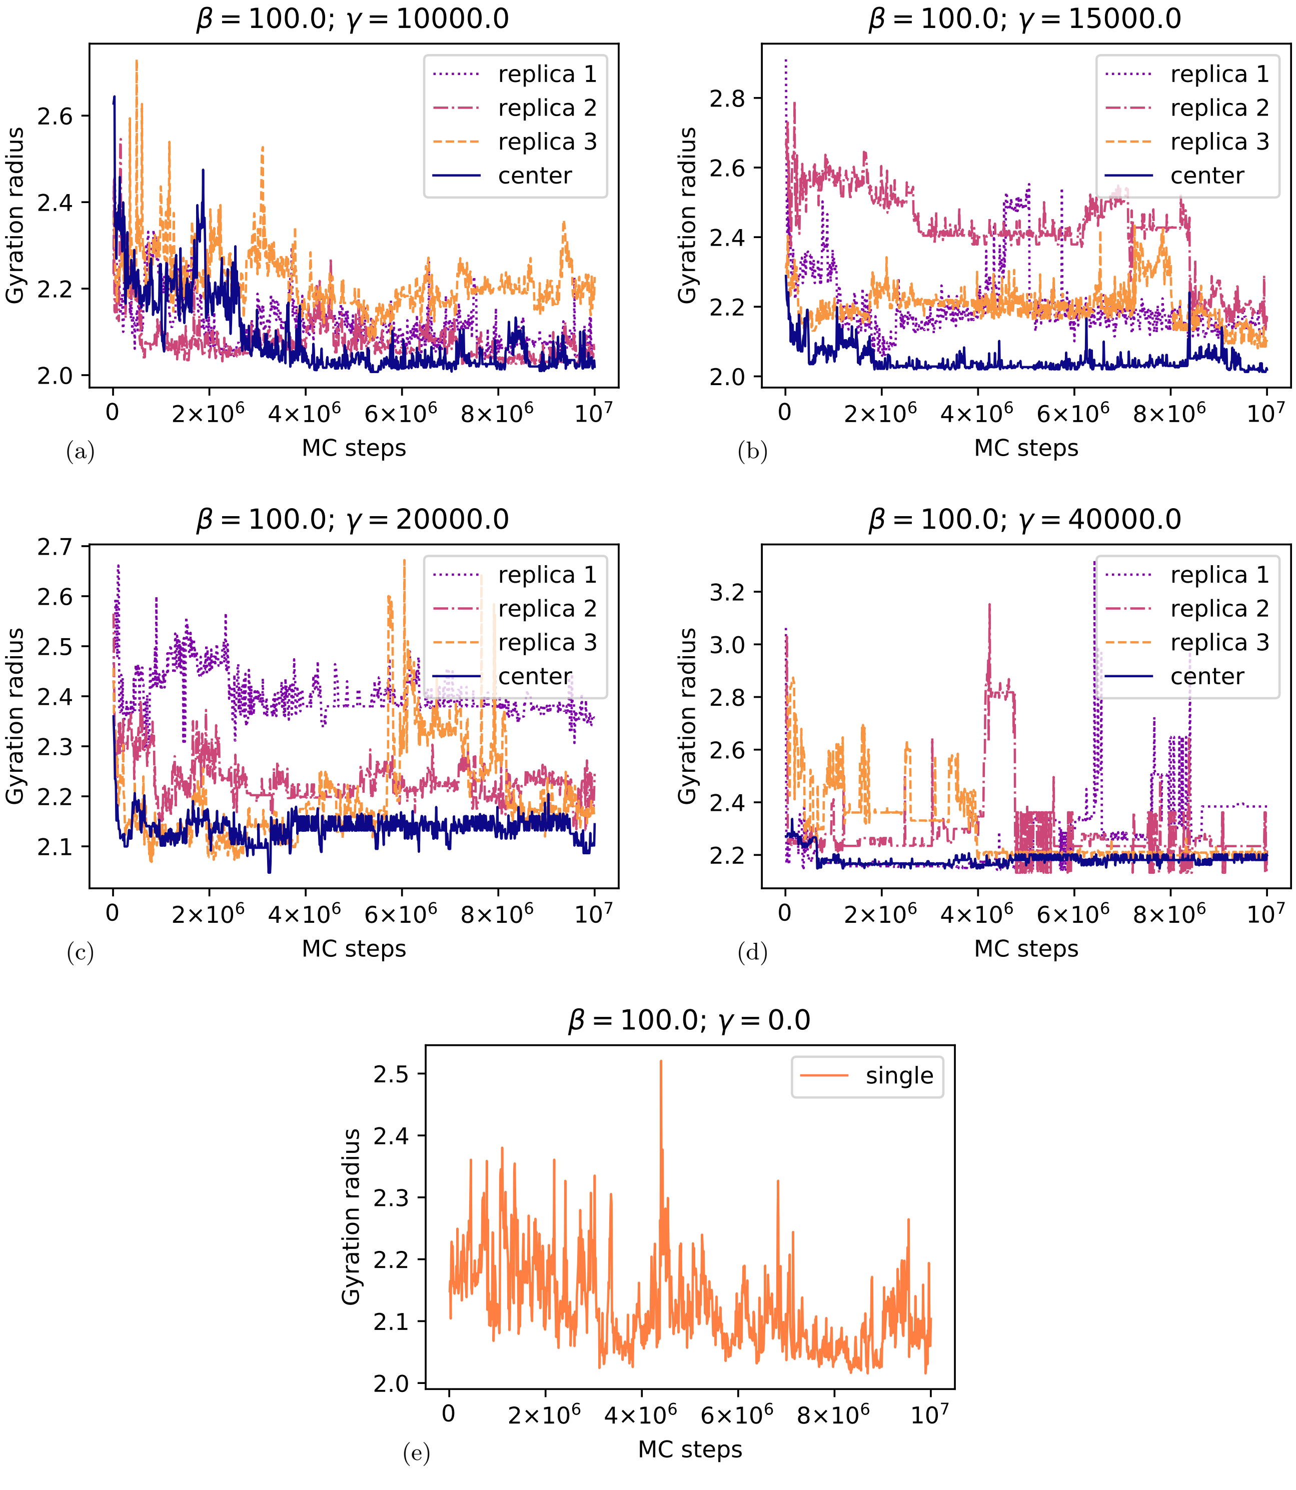


FIG. S1: **Examples of trajectories of the gyration radius.** (a-d) The solid blue curve corresponds to the gyration radius of the center, while the other curves correspond to the radius of the three replicas. (e) The curve corresponds to the gyration radius of a single configuration obtained with plain Monte Carlo. The radius of gyration is recorder every $10^4$ MC steps. To compute the thermal averages of the phase diagram in Fig. 1a of the main text we used the last 300 samples of the trajectory of the center (namely from MC steps $> 7 \cdot 10^6$ to the end of the trajectory). We observe that the radius of the centers has lower variability than the one of plain Monte Carlo and it decreases faster.

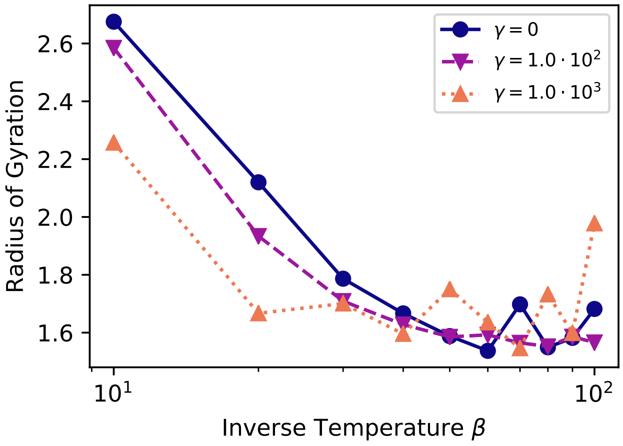


FIG. S2: **The phase diagram is consistent with respect to choices of distance and replica coupling scheme**. This portion of the phase diagram has been computed using Root Mean Square Distance (RMSD) as distance and by coupling replicas with each other, without a center. RMSD between two polymers is calculated as $d_{\mathrm{RMDS}}(\Gamma, \Gamma') = \frac{1}{N}(\sum_{i=1}^{N} ||\vec{r_i}^{\Gamma} - \vec{r_i}^{\Gamma'}||^2)^{1/2}$, where $N$ is the number of residues and $\vec{r_i}^{\Gamma}$ is the position of the $i$-th residue of the structure $^{\Gamma}$. The effects of local entropy on the transition with these choices are qualitatively the same as in Fig. 1 of the main text.

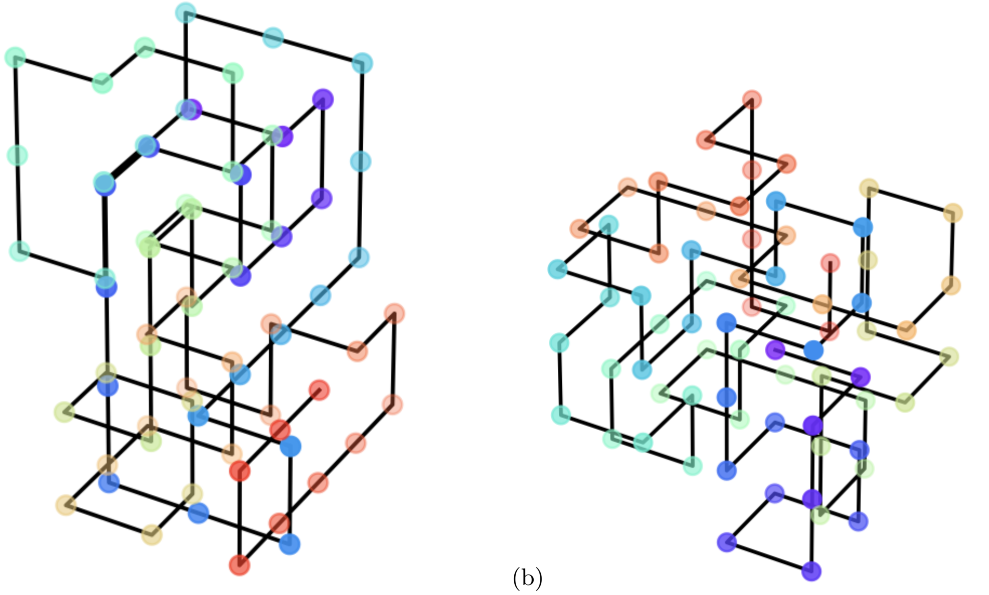

(a) (b)

FIG. S3: **Examples of compact configurations in the lattice model.** Panel (a) is obtained with plain Monte Carlo, panel (b) is obtained by sampling local entropy. The color of the beads represents the index of each bead, from 0 (red) to 70 (purple).

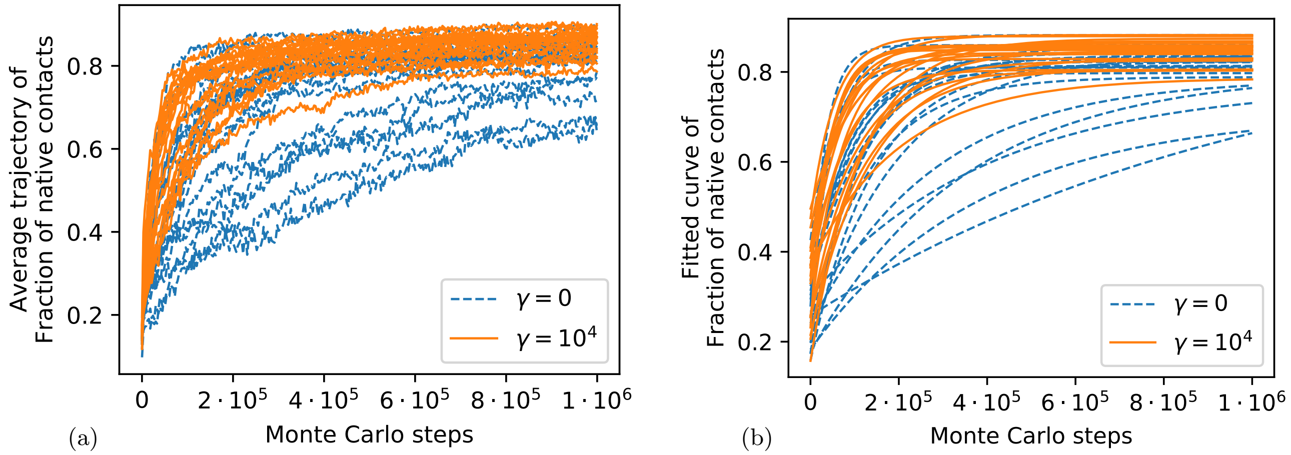


FIG. S4: **Examples of averaged folding trajectories of lattice Go models and corresponding fitted curves.** The left panel shows trajectories of the fraction of native contacts as a function of Monte Carlo steps. The blue dashed ones correspond to references with $\gamma = 0$, the orange solid ones correspond to references with $\gamma = 1e4$. The right panel shows the corresponding curves obtained by fitting the trajectories with an exponential curve.

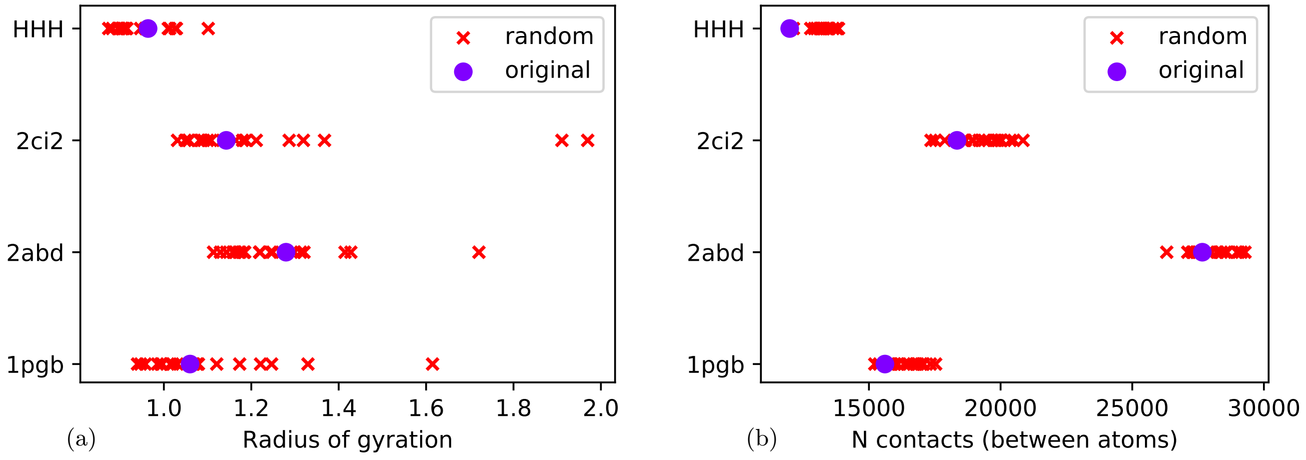


FIG. S5: **The decoys have similar compactness than the native structures.** We show radius of gyration and number of atomic contacts for the proteins under study and for the associated random decoys. In order to obtain this distribution of properties for decoy configurations we set $C_{ij}^{(6)} = 1.4 \cdot 10^{-2}\,\mathrm{kJ\,mol^{-1}\,nm^6}$ and $C_{ij}^{(12)} = 1.0 \cdot 10^{-4}\,\mathrm{kJ\,mol^{-1}\,nm^6}$ in the Lennard-Jones potentials between pairs of atoms.

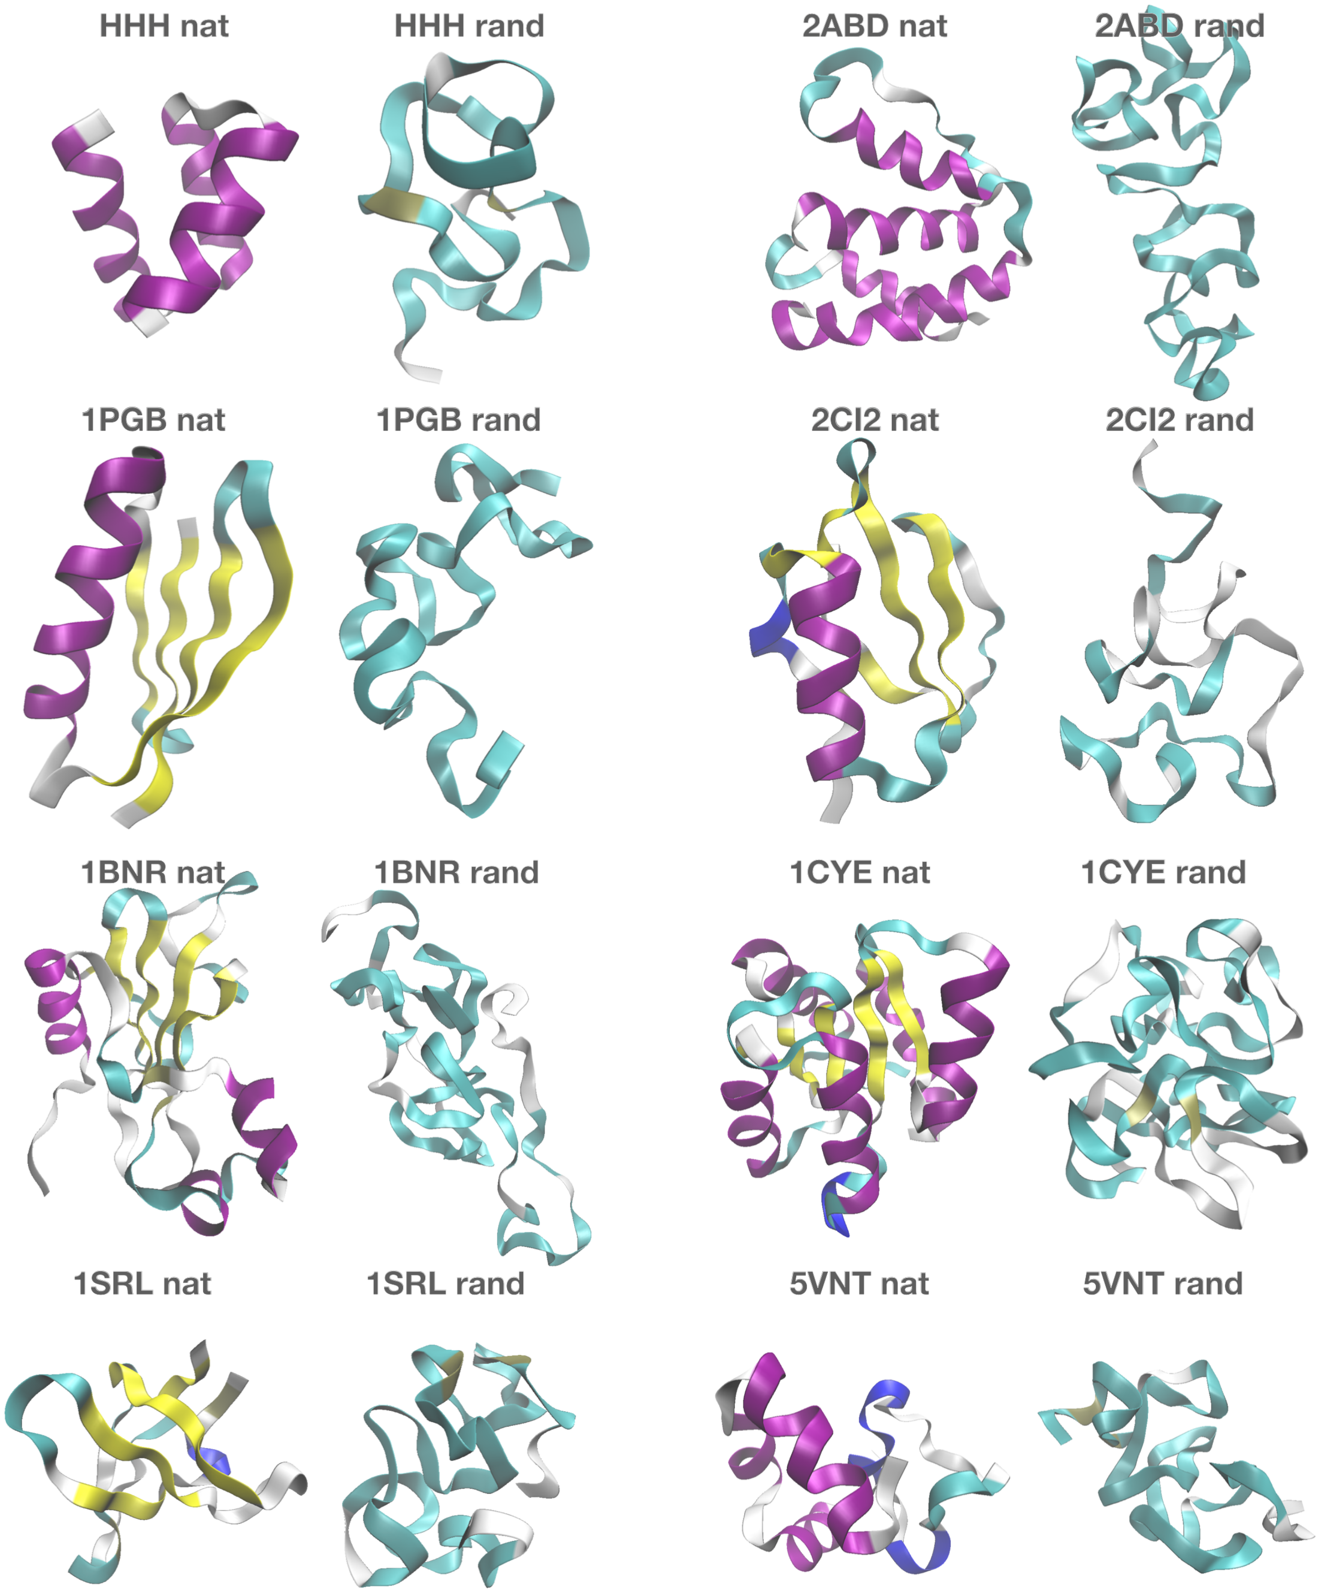


FIG. S6: **Examples of compact configurations in the all-atom model.** Different colors correspond to secondary structures, showing that random decoys show little to no secondary content.

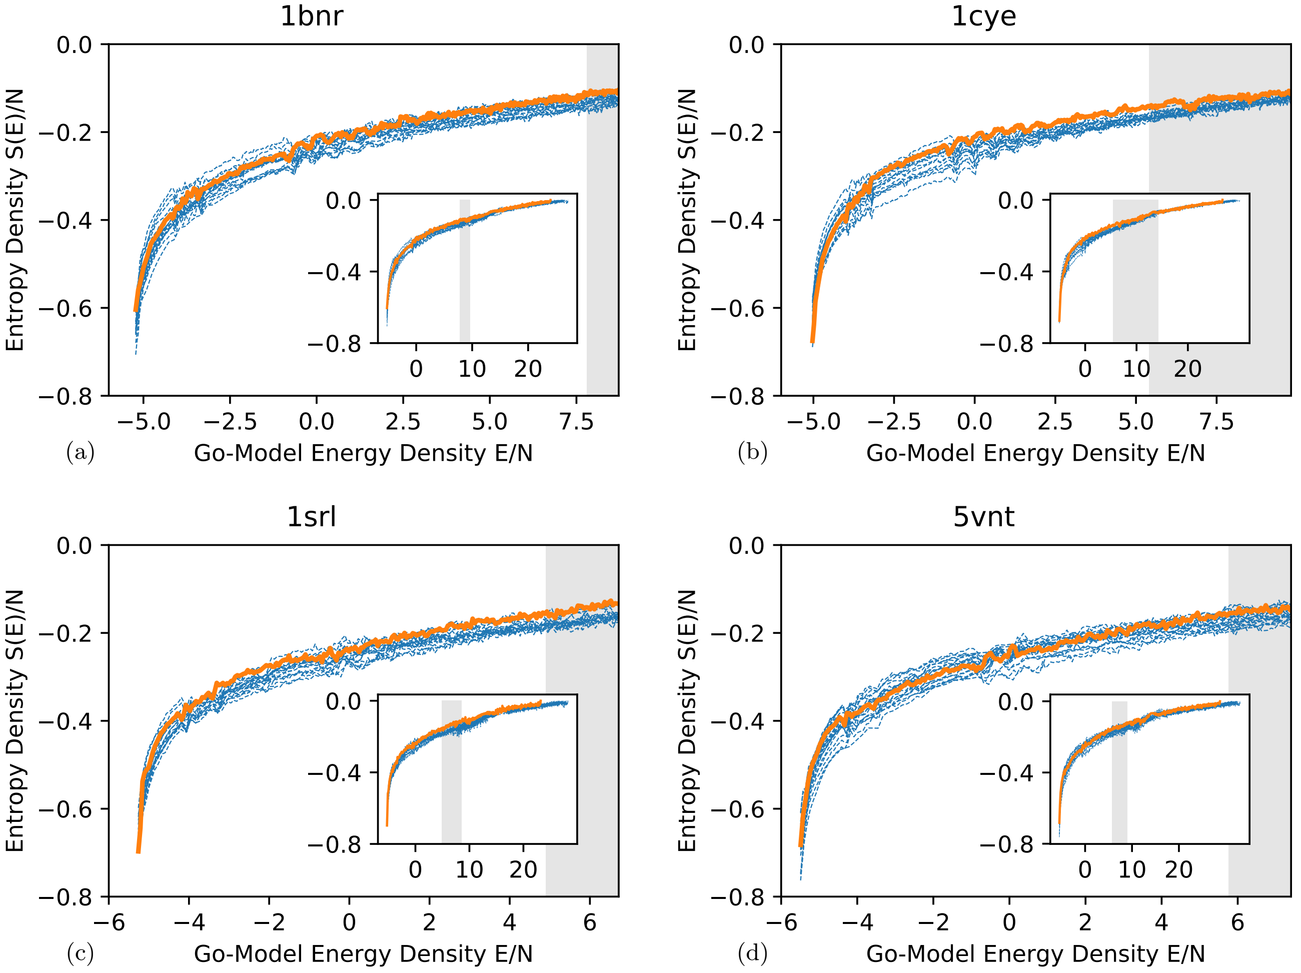


FIG. S7: **Entropy curves for the four proteins not shown in the main text.**

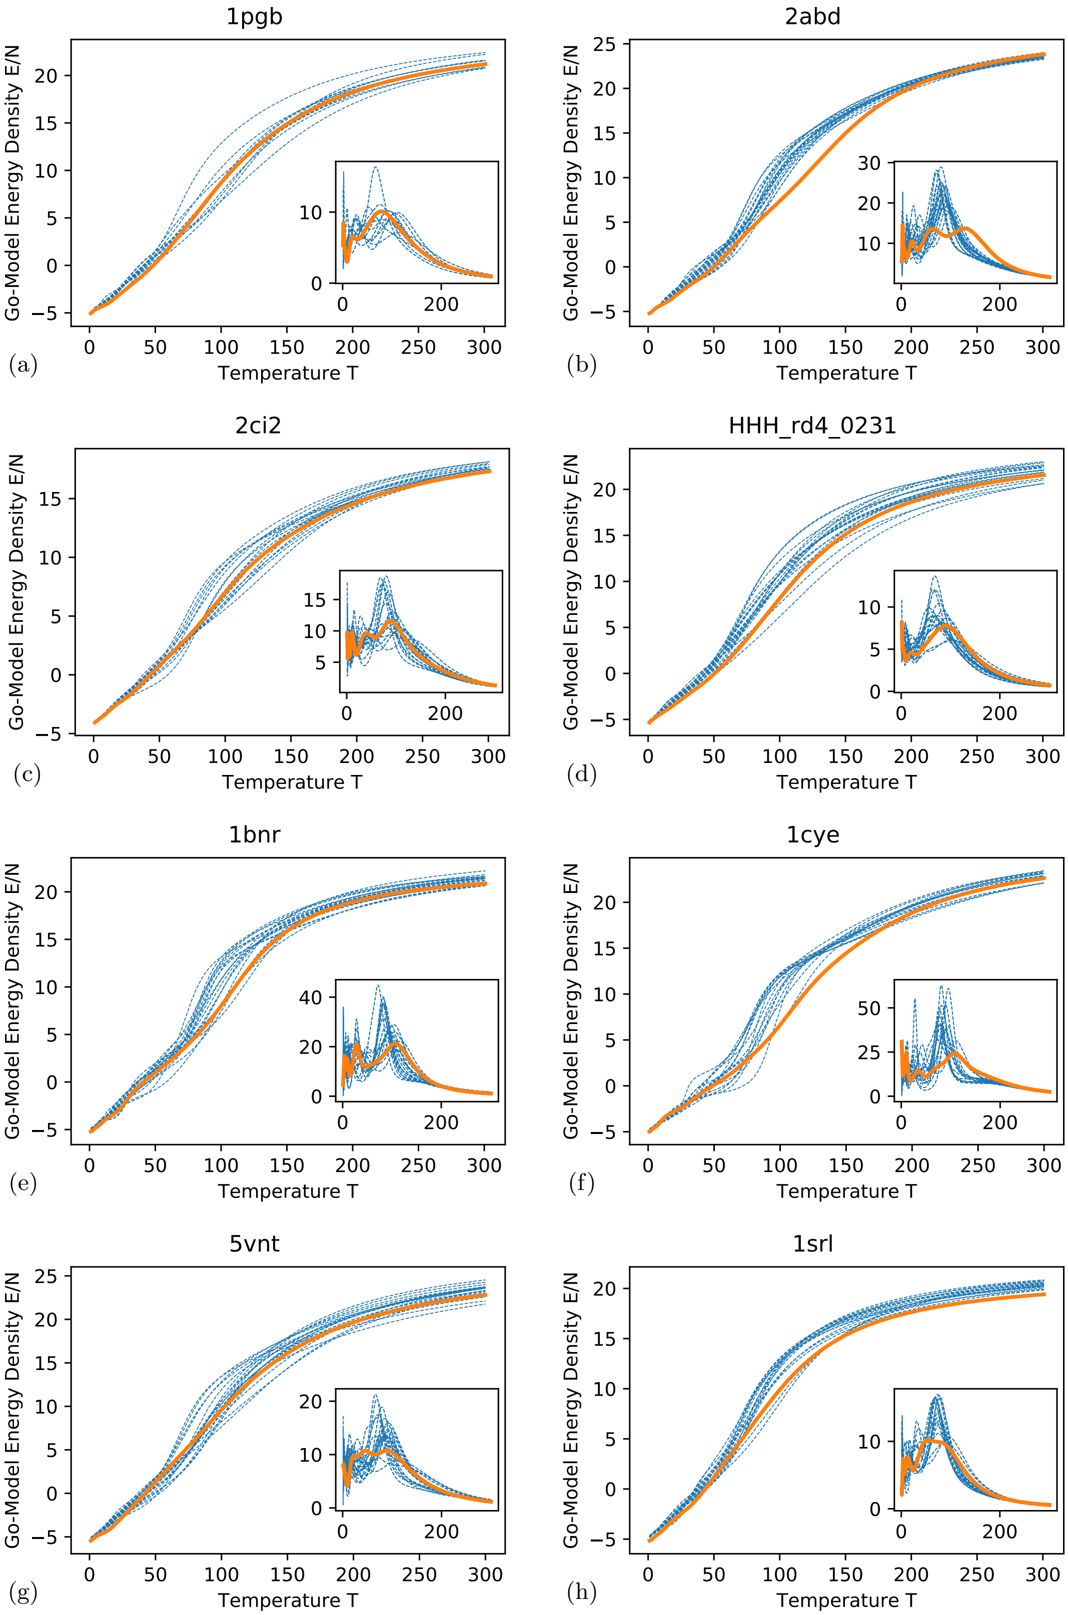


FIG. S8: **Thermodynamics of all-atom models.** Each plot show the internal energy and the specific heat (inset) as a function of the temperature for the four proteins we studied (solid orange curves) and for their random decoys (dashed blue curves).
